# Supplementary material for: Estimating Entropy of Distributions in Constant Space
Source: arXiv:1911.07976 source file (2019-11-18)
Supplement: Supplementary file 1 [file supp.tex]

\documentclass{article}

% if you need to pass options to natbib, use, e.g.:
%     \PassOptionsToPackage{numbers, compress}{natbib}
% before loading neurips_2019

% ready for submission
% \usepackage{neurips_2019}

% to compile a preprint version, e.g., for submission to arXiv, add add the
% [preprint] option:
%     \usepackage[preprint]{neurips_2019}

% to compile a camera-ready version, add the [final] option, e.g.:
\usepackage{neurips_2019}

% to avoid loading the natbib package, add option nonatbib:
%     \usepackage[nonatbib]{neurips_2019}

\usepackage[utf8]{inputenc} % allow utf-8 input
\usepackage[T1]{fontenc}    % use 8-bit T1 fonts
\usepackage{hyperref}       % hyperlinks
\usepackage{url}            % simple URL typesetting
\usepackage{booktabs}       % professional-quality tables
\usepackage{amsfonts}       % blackboard math symbols
\usepackage{nicefrac}       % compact symbols for 1/2, etc.
\usepackage{microtype}      % microtypography
\usepackage[english]{babel}
\usepackage{enumitem,bbm,verbatim,amscd,float,mathtools}
\usepackage[normalem]{ulem}
\usepackage{amsthm}
\usepackage{amsmath, amssymb, graphicx, url, algorithm}
\usepackage[noend]{algpseudocode}
\usepackage{times}
\input{glodef}
\input{locdef}

\title{Estimating Entropy of Distributions in Constant Space}

% The \author macro works with any number of authors. There are two commands
% used to separate the names and addresses of multiple authors: \And and \AND.
%
% Using \And between authors leaves it to LaTeX to determine where to break the
% lines. Using \AND forces a line break at that point. So, if LaTeX puts 3 of 4
% authors names on the first line, and the last on the second line, try using
% \AND instead of \And before the third author name.

\author{
  Jayadev Acharya\\
  Cornell University \\
  \texttt{acharya@cornell.edu} \\
  % examples of more authors
  \And
  Sourbh Bhadane \\
  Cornell University\\
  \texttt{snb62@cornell.edu} \\
  \And 
  Piotr Indyk\\
  Massachusetts Institute of Technology\\
  \texttt{indyk@mit.edu} \\
  \And
  Ziteng Sun\\
  Cornell University\\
  \texttt{zs335@cornell.edu}\\
  % Address \\
  % \texttt{email} \\
  % \AND
  % Coauthor \\
  % Affiliation \\
  % Address \\
  % \texttt{email} \\
  % \And
  % Coauthor \\
  % Affiliation \\
  % Address \\
  % \texttt{email} \\
  % \And
  % Coauthor \\
  % Affiliation \\
  % Address \\
  % \texttt{email} \\
}

\begin{document}

\maketitle

\begin{abstract}
  We consider the task of estimating entropy of $k$-ary distributions from samples in the streaming model, where space is limited. Our main contribution is an algorithm that takes
$	O\Paren{\frac{k \log (1/\varepsilon)^2}{\varepsilon^3}}$ 	samples and using $O(1)$ memory words, obtains a $\pm\varepsilon$ estimate of $H(p)$. Without space limitations, the sample complexity has been established as $S(k,\varepsilon)=\Theta\left(\frac k{\varepsilon\log k}+\frac{\log^2 k}{\varepsilon^2}\right)$, which is sub-linear in the domain size $k$. All current sample-optimal estimators also require nearly-linear space in $k$.
	
	Our algorithm partitions $[0,1]$ into intervals and estimates the entropy contribution of probabilities in each interval. The intervals are designed to trade the bias and variance within each interval.
	
	Distribution property estimation and testing with limited memory is a largely unexplored research area, and we hope that our work will spur many works in this field.
\end{abstract}
\section{Introduction}
\input{intro.tex}

\subsection{Problem Formulation}
\input{formulation.tex}

\subsection{Prior Work}
\input{related-work.tex}

\input{preliminaries}
\input{one-interval.tex}

\section{Interval-based Algorithms}\label{sec:interval}
\input{two-intervals.tex}
\input{general-algorithm.tex}

\section{Open Problems}
There are several interesting questions that arise from our work. Perhaps the most interesting, and challenging are proving lower bounds for space requirements for entropy estimation. Is it possible to design a sample-optimal algorithm with $poly(\log k)$ space? We hope our work encourages research into other distribution testing and property estimation problems in the streaming model. 

\bibliographystyle{unsrt}
\bibliography{masterref}

\appendix  

\input{app:proofs-simple.tex}

\section{Proofs from Section~\ref{sec:simplealgo}}\label{sec:mdlpfs}
\subsection{Proof of Lemma~\ref{lem:mdlbias} : Bias Bound}
From Algorithm~\ref{alg1}, we can express $\bar{H}$ as 
 \begin{align*}
 \bar{H} &= \frac{1}{\vSmp}\sum\limits_{t=1}^{\vSmp} \sum\limits_{x\in \mathcal{X}} \indctr{ x = x_t }\log \left( \frac{\bSmp}{N_{x_t} + 1} \right). \\
 &=  \sum\limits_{x\in \mathcal{X}} \frac{1}{\vSmp}\sum\limits_{t=1}^{\vSmp} \indctr{ x = x_t }\log \left( \frac{\bSmp}{N_{x_t} + 1} \right).
 \end{align*}
 The above formulation can be thought of as an empirical average of $\log\left( \frac{\bSmp}{N_X+1} \right)$, where $X \sim p$. 
Therefore, 

\begin{equation}
\Expc{\bar{H}} =\sum\limits_{x \in \mathcal{X}} p\left( x \right) \Expc{ \log \left( \frac{\bSmp}{N_{x}+1} \right)}.
\end{equation}

% Therefore,
%\begin{align*}
%\Expc{\bar{H}} &=\frac{1}{\vSmp} \sum\limits_{t=1}^{\vSmp} \sum\limits_{x \in \mathcal{X}} \Expc{ \indctr{x = x_t} \log \left( \frac{\bSmp}{N_{x_t}+1} \right) }\\
%&= \frac{1}{\vSmp} \sum\limits_{t=1}^{\vSmp} \sum\limits_{x \in \mathcal{X}} p\left(x\right) \Expc{ \log \left( \frac{\bSmp}{N_{x_t}+1} \right) \mid x_t = x }.
%\end{align*} 
%Note that, given $x_t = x$, $N_{x_t} \sim \text{Bin} \left(\bSmp,p\left(x\right) \right)$. We drop the conditional expectation and denote $N_{x_t}$ as $N_{x,x_t}$ from now.
%\begin{equation*}
%\Expc{\bar{H}} =\frac{1}{\vSmp} \sum\limits_{t=1}^{\vSmp} \sum\limits_{x \in \mathcal{X}} p\left(x\right)\Expc{ \log \left( \frac{\bSmp}{N_{x,x_t} + 1} \right)}.
%\end{equation*}

\begin{align}
\Ent{p} -  \Expc{ \bar{H}} &= \sum\limits_{x \in \mathcal{X}} p\left(x\right) \log \frac{1}{p\left(x\right)} - \sum\limits_{x\in \mathcal{X}} p\left(x\right)\Expc{\log \left( \frac{\bSmp}{N_{x}+1} \right)} \nonumber \\
&= \sum\limits_{x \in \mathcal{X}} p\left(x \right) \Expc{ \log \left( \frac{N_{x}+1}{\bSmp p\left(x\right)} \right)}  \nonumber \\
&\leq \sum\limits_{x \in \mathcal{X}} p\left(x \right)  \log \left( \Expc{\frac{N_{x}+1}{\bSmp p\left(x\right)}}  \right) \label{eq:modelJens} \\
&= \sum\limits_{x \in \mathcal{X}} p\left(x \right)  \log \left( 1 + \frac{1}{\bSmp p\left(x\right)} \right) \nonumber \\
&\leq \frac{k}{\bSmp}. \label{eq:logineq}
\end{align}
where we obtain \eqref{eq:modelJens} using Jensen's inequality and \eqref{eq:logineq} follows from $\log \left(1+x \right) \leq x$. We now bound $\Expc{\bar{H}} - \Ent{p}$.

\begin{align}
\Expc{\bar{H}} - \Ent{p} &= \sum\limits_{x \in \mathcal{X}} p\left(x \right) \Expc{\log \left( \frac{\bSmp p\left(x\right)}{N_{x}+1} \right)} \nonumber \\
&\leq \sum\limits_{x \in \mathcal{X}} p\left(x \right)  \log \left( \Expc{\frac{\bSmp p\left(x\right)}{N_{x}+1}} \right) \label{eq:mdlJens}\\
&\leq  \sum\limits_{x \in \mathcal{X}} p\left(x \right) \log \left( \frac{\bSmp}{\bSmp+1} \right) < 0. \label{eq:invbinom}
\end{align}
where \eqref{eq:mdlJens} is obtained using Jensen's inequality and \eqref{eq:invbinom} follows from  Lemma~\ref{binreciplemma}. Therefore,
\begin{equation} \label{bias}
\lvert \Expc{\bar{H}} - \Ent{p} \rvert \leq \dfrac{k}{\bSmp} .
\end{equation} 

\section{Two interval Algorithm Proofs}\label{sec:twointproofs}

\input{two-intervalspf.tex}

\section{General Interval Algorithm} \label{pf:thm:general}
\subsection{General Interval Algorithms}
\label{app:general-algorithms}
We provide the pseudocode of the various procedures for our main algorithms in this section. 

Algorithm~\ref{alg:interval-general} is the interval estimation algorithm that tests from samples where a $p(x)$ belongs to a certain interval $I_t$. 

\begin{algorithm}[h]
		\caption{Estimating intervals: General Case : \textsc{GenEstInt}$(\bset{t},x)$} \label{alg:interval-general}
		\begin{algorithmic}[1]
			\Require $\bset{t},x$ drawn from $p$
			\For{$i = 1 \text{ to } t  $}
			\State Generate $\bSmp_i$ samples from $p$ 
			\State {\textbf{if} $x$ appears more than $\bSmp_i \ell_i$ times  \textbf{then} Output $I_i$}
			\EndFor
			%\State Generate $\bSmp_t$ samples from $p$ 
			%\State {\textbf{if} $x$ appears more than $\bSmp_t \ell_t$ times \textbf{then} Output $I_t$}
			%\State{\textbf{else} Output $I_T$}
			\State Output $I_T$
		\end{algorithmic}
	\end{algorithm}

Algorithm~\ref{alg:estp_general} describes the procedure to estimate $\p_\cA(I_t)$'s. 
\begin{algorithm}[h]
 	\caption{Estimating $p_\cA\left(I_i \right),1 \leq i \leq T-1$ : \textsc{GenEstProbInt}$(\bset{T-1},\vset{T-1})$ } \label{alg:estp_general}
 	\begin{algorithmic}[1]
 	\Require $\bset{T-1},\vset{T-1}$
 		\For{$i = 1, 2, ..., T-1$}
 		\State $\hat{p}_\cA\left(I_i\right) = 0$
 		\For{$t = 1 \text{ to } \vSmp_i$}
 		\State Sample $x \sim \p$.
 		\State{\textbf{if} $\textsc{GenEstInt}\left(\left \lbrace \bSmp_j \right \rbrace_{j = 1}^{i} , x\right) = I_i$ \textbf{then} $\hat{p}_\cA\left(I_i \right)= \hat{p}_\cA\left(I_i \right)+ \frac{1}{\vSmp_i}$}	
 		\EndFor
 		\EndFor
 		%$\hat{p}_{\cA} \left(I_T\right) = 1 - \sum\limits_{i=1}^{T-1} 	\hat{p}_{\cA} \left(I_i\right)$
 	\end{algorithmic}
 \end{algorithm} 

Algorithm~\ref{alg:esth_general} estimates the entropy contributions from the intervals. 
\begin{algorithm}[h]
	\caption{Estimating ${H}_i$'s : \textsc{GenCondExp}$\left( \bset{T}, \vset{T} \right)$} \label{alg:esth_general}
	\begin{algorithmic}[1]
	\Require $\bset{T},\vset{T}$
		\For{$i=1 \text{ to } T$}
		\State $\hat{H}_i = 0, S_i = 0$
		\For{$t = 1 \text{ to } \vSmp_i$}
		\State Generate $x \sim p$
		\If{$\textsc{GenEstInt}\left(\left \lbrace \bSmp_j \right \rbrace_{j = 1}^{i}, x\right)$is $I_i$}
		\State $S_i = S_i + 1$
		\State Let $N_{x,i} \leftarrow$ \# occurrences of $x$  in the next $\bSmp_i$ samples
		\State $E_{x,i} = \max \{ \log \left(\frac{\bSmp_i}{N_{x,i} + 1} \right), \log \frac{1}{4h_i}\} $ \label{clipping_gen}
		\State $\hat{H}_i = \hat{H}_i +E_{x,i} $ 
		\EndIf
		\EndFor
		\State $\bar{H}_i = \frac{\hat{H}_i}{S_i}$
		\EndFor
		%	\State Output  $\hat{H} = \sum_{i = 1}^{T - 1}\hat{p}\left[I_i\right] \hat{H_i} + \left(1-\sum_{i = 1}^{T - 1} \hat{p}\left[I_i\right]\right) \hat{H_T}$
	\end{algorithmic}
\end{algorithm}

\subsection{Unclipped Bias Bound} \label{sec:bias}
\input{general-bias.tex}
\subsection{Clipping Error Bound}\label{sec:clip}

\input{general-clipping.tex}
\subsection{Concentration Bound} \label{sec:var}
\input{general-variance.tex}

\end{document}
